# Supplementary material for: Where is Physical RSI capability from? An Observational Scaling Law of LLM-as-policy
Source: arXiv:2610.26848 source file (2026-10-19)
Supplement: Supplementary file 1 [file X_suppl.tex]

\clearpage

%% Supplementary material. Column order in every table and four-number list: Astra / Sol / Opus / Sonnet
%% (GPT-6 Astra, GPT-6.1 Sol, Claude Opus 5.5, Claude Sonnet 5.5).
%% All CIs: paired task bootstrap over the 18 tasks, B = 5000, seed 20261012, percentile 95%.
%% Division of labor with the body (2026-10-13 trim): the body keeps one defining formula per axis,
%% the notation paragraph, the tool interface and the headline numbers; this appendix keeps only what the
%% body dropped or pointed here (task table, protocol rules and budgets, per-system heterogeneity, axis
%% identities and robustness tables, per-task and per-round results, cost readings, frozen held-out tests,
%% and the pending PCA framework).

\section{Benchmark Details}
\label{app:benchmark}

\Cref{tab:app-tasks} lists the 18 tasks with their native step limits, scoring modes and success criteria. Scoring modes: \emph{binary} = success or failure only (score 0 or 1); \emph{transition} = ordered partial-credit tiers, the score is the value of the highest tier reached; \emph{count-trigger} = the tier is assigned by counting satisfied sub-conditions at a trigger instant. Every success check is evaluated independently of the partial score; in most multi-object tasks success additionally requires both arms back at the home pose, whereas partial tiers require only open grippers. Control runs at 25\,Hz (control step 0.04\,s), so a step limit of 300--1300 corresponds to 12--52\,s of simulated motion. In the 18-task benchmark every round uses the native default layout (scene seed 0); layout variants 1--17 exist only for the six ablation tasks (\cref{app:additional}).

The success criteria in~\cref{tab:app-tasks} paraphrase the task reward code; thresholds such as the push-T tolerance ($\le 7$\,mm, $\le 7^\circ$) were decoded from the scoring code and .

\begin{table*}[tp]
  \caption{\textbf{The 18 \methodname tasks with step limits, scoring modes and success criteria.} Partial-credit tiers are given in percent of the native score; $i$ of $n$ denotes the tier reached when $i$ of $n$ objects satisfy the stage condition with grippers open. ``Arms home'' = both arms back at the origin pose.}
  \label{tab:app-tasks}
  \tablestyle{2.5pt}{1.08}
  \scriptsize
  \begin{tabular}{y{8} y{84} z{22} y{66} y{158} y{92}}
    \toprule
    \# & Task & Steps & Scoring (tiers, \%) & Success criterion & Partial-credit stages \\
    \midrule
    1 & \texttt{arrange\_largest\_number} & 1050 & transition; 4 digits [5,15,30,100], 5 digits [5,15,25,40,100] & Every digit block on the mat of its rank in descending-digit order ($xy\le 2$\,cm), readable orientation ($45^\circ$ tolerance; symmetric relaxations for 0 and 8); arms home. & $i$ of $n$ digits placed. \\
    2 & \texttt{classify\_objects\_by\_language} & 1100 & transition [10,40,100] & All objects of each of three instructed categories inside their basket, below the rim ($z\le$ rim $+1$\,cm); arms home. & $i$ categories fully sorted with no foreign object in that basket. \\
    3 & \texttt{cover\_blocks} & 800 & transition [0,0,5,15,30,100] & Sequential: cover the left block, then left$+$middle, then all three (cups inverted within $10^\circ$); then uncover red, green, blue; arms home. Fails if any block moves $>5$\,cm. & Stage chain; the first two tiers score 0, so a 0 can mean stage 0, 1 or 2. \\
    4 & \texttt{deposit\_coin} & 300 & transition [20,100] & Coin bounding box inside the piggy bank between its bottom and center tags; arms home. & Coin lifted $\ge 8$\,cm $\to 0.2$. \\
    5 & \texttt{fill\_pen\_holder} & 1100 & transition [10,25,40,90] & All 4 pens within 3.5\,cm of the holder axis, inserted $\ge 3.5$\,cm, tip down; holder upright; arms home. & $i$ pens inserted within $45^\circ$ of vertical, holder within $45^\circ$ of upright. Top tier is 0.9. \\
    6 & \texttt{insert\_key} & 300 & transition [15,100] & Key $\ge 2.5$\,cm deep in the slot, $xy$ offset $\le 7$\,mm, vertical within $7^\circ$, turned within $30^\circ$ of the $60^\circ$ target; no arm-home requirement. & Key lifted $\ge 5$\,cm $\to 0.15$. \\
    7 & \texttt{match\_and\_pick\_from\_conveyor} & 700 & binary & The object matching the first conveyor object is lifted $\ge 10$\,cm. & --- \\
    8 & \texttt{organize\_table} & 1000 & transition [25,50,75,100] & Mouse on the mouse pad, keyboard inside the frame, figurine on the stand, alarm clock on the drawer top, each upright and stationary ($<2$\,mm); arms home. & $i$ of 4 items placed and still. \\
    9 & \texttt{pack\_objects\_into\_box} & 1300 & transition [10,25,50,100] & Car, toothbrush, hammer and shoe inside the box, aligned with its long axis ($45^\circ$), front side facing left ($60^\circ$); box upright (long axis within $40^\circ$ of $x$); arms home. & Box aligned $+\,i$ items packed. \\
    10 & \texttt{play\_Xylophone} & 500 & binary & Mallet head strikes keys 1--8 from left to right (1--3.6\,cm above each hit point, lifted $\ge 2.5$\,cm in between); no arm-home requirement. & --- \\
    11 & \texttt{plug\_in\_charger} & 400 & binary & Charger $\ge 1.5$\,cm deep inside the socket footprint, axis within $10^\circ$ of the socket normal; arms home. & --- \\
    12 & \texttt{pour\_by\_language} & 800 & count-trigger [20,50,100] & For each of three color-matched bottle/bowl pairs, $\ge 95\%$ of the liquid is in its bowl when the bottle returns upright ($30^\circ$), in order bowl 0 $\to$ 1 $\to$ 2; scored only when both arms return home. & Bowl 0 $\to 0.2$; bowls 0$+$1 $\to 0.5$; poured but arms not home $\to 0$. \\
    13 & \texttt{pour\_liquid\_into\_cup} & 400 & binary & $\ge 97\%$ of the liquid particles in the cup when the bottle returns upright ($30^\circ$); no arm-home requirement. & --- \\
    14 & \texttt{push\_T} & 600 & binary & T-block pose matches the target pad (position $\le 7$\,mm, angle $\le 7^\circ$); arms home. Fails if the T is lifted $>1$\,cm. & --- \\
    15 & \texttt{put\_bottles\_into\_dustbin} & 700 & transition [10,25,40,100] & All 4 bottles resting on the dustbin bottom (0--40\,cm above it); arms home. & $i$ bottles in. \\
    16 & \texttt{stack\_blocks\_by\_language} & 400 & transition [20,100] & Three blocks stacked in the instructed color order ($xy\le 1.75$\,cm); arms home. & Bottom two stacked in order, bottom block not lifted $\to 0.2$. \\
    17 & \texttt{store\_tools\_in\_toolbox} & 900 & transition [25,50,75,100] & Pliers, hammer, tape measure and wrench each at its slot, aligned, and covered by the closed lid; arms home. & $i$ tools in slot and covered (orientation not checked). \\
    18 & \texttt{swap\_blocks} & 700 & binary & Sequential: move block A to the empty mat, press the button, move B to A's mat, press, move A to B's mat, press; both blocks on swapped mats ($\le 3$\,cm); final press; arms home. Fails after more than 3 presses. & --- \\
    \bottomrule
  \end{tabular}
\end{table*}

\paragraph{Task sets used by the metrics.} The graded set $\mathcal{G}$ (12 tasks with partial-credit tiers) is the complement of the six binary tasks (7, 10, 11, 13, 14, 18). The frozen common-success set $\mathcal{I}$ used by D6 contains the nine tasks solved by all four systems: \texttt{arrange\_largest\_number}, \texttt{classify\_objects\_by\_language}, \texttt{cover\_blocks}, \texttt{match\_and\_pick\_from\_conveyor}, \texttt{pour\_by\_language}, \texttt{pour\_liquid\_into\_cup}, \texttt{push\_T}, \texttt{put\_bottles\_into\_dustbin}, \texttt{stack\_blocks\_by\_language}.

\section{Protocol Details}
\label{app:protocol}

\paragraph{Actions and observations.} An action sets a target pose for each end-effector, within 5\,cm translation and 0.35\,rad rotation of its current pose per call, executed for 1--5 control steps at 25\,Hz; each call returns a state JSON and three camera images (\texttt{cam\_high}, \texttt{cam\_left\_wrist}, \texttt{cam\_right\_wrist}; JPEG $q{=}90$, PNG originals for Astra).

\paragraph{Zero-shot round (K0).} K0 is run once per task as the zero-shot baseline and is not part of the self-improvement chain; Astra's K0 results were reused from an earlier run under the Context protocol.

\paragraph{Stop, retry and invalid-round rules.} The round cap is 17; a chain stops at the first native success with no confirmation round. If the revision cannot be completed within the same session, the round is withdrawn and rerun at the same round index. Rounds without a valid grade (\eg a client failure before the episode started) do not consume a round index and are rerun at the same $k$, at most three times per round; rounds whose action outcome is unknown are not replayed. Rounds ended by the inference-time limit count as failures; in D7 their unexecuted steps are charged at the full step limit. Opus and Sonnet chains were allowed to run to K20, but every cross-system number truncates at K17 (Sonnet's K19 success on \texttt{deposit\_coin} is excluded).

\paragraph{Budgets.} Inference budget 4200\,s per round; revision budget 1800\,s (Astra, Sol) or 600\,s (Opus, Sonnet) after grading; program execution in the workspace has no total time limit, but a program is killed after 700\,s without output and without a tool reply. The physical budget per task is $17\,N_t$, \ie 17 full-step-limit attempts.

\begin{table*}[t]
  \caption{\textbf{Per-system configuration and known protocol heterogeneity.} The systems are ``model + configuration'' pairs; all cross-system comparisons in the paper are descriptive.}
  \label{tab:app-config}
  \tablestyle{4pt}{1.1}
  \begin{tabular}{p{128pt} y{74} y{74} y{72} y{72}}
    \toprule
    Item & Astra & Sol & Opus & Sonnet \\
    \midrule
    Model & GPT-6 Astra & GPT-6.1 Sol & Claude Opus 5.5 & Claude Sonnet 5.5 \\
    Client & Codex CLI 0.156.1 & Codex CLI 0.162.0 & Claude Code & Claude Code \\
    Reasoning effort & xhigh & xhigh & high & xhigh \\
    Round cap (analyzed) & 17 (17) & 17 (17) & 20 (17) & 20 (17) \\
    Revision window & 1800\,s & 1800\,s & 600\,s & 600\,s \\
    Observation images & PNG & JPEG $q$90 & JPEG $q$90 & JPEG $q$90 \\
    Extra task hints & 3 tasks\textsuperscript{a} & none & none & none \\
    Canonical episodes (K0 + K1--K17) & 18 + 91 & 18 + 143 & 18 + 175 & 18 + 165 \\
    Known extra attempts & 13 & 9 & 21 & 37 \\
    K0 episodes ended by time limit &  &  & 11 & 6 \\
    K1 episodes ended by time limit &  &  & 9 &  \\
    Failed K1--K17 rounds ended by time limit & 5 & 0 & 14 & 2 \\
    Unfinished chains at K17 & 0 & 0 & 0 & 3 \\
    \bottomrule
  \end{tabular}
  \par\smallskip\footnotesize \textsuperscript{a}Scoring-structure and revision-hygiene notes on \texttt{pack\_objects\_into\_box} (from K7), \texttt{store\_tools\_in\_toolbox} (K8) and \texttt{swap\_blocks} (K12). Astra's harness code changed mid-run (v196--v206; Sol ran v210), and its per-round ledger was rebuilt from a rescue index (104 graded attempts $\to$ 91 canonical rounds $+$ 13 extra attempts).
\end{table*}

\paragraph{Heterogeneity.} \Cref{tab:app-config} collects the configuration differences that must accompany any cross-system statement, together with the per-system split of the 646 canonical episodes. Reasoning-clock definitions, token meters and timing boundaries differ by vendor; wall-clock is per-episode native time summed over parallel runs and is neither calendar time nor inference latency.

\section{Metric Details}
\label{app:metrics}

Notation is as in~\cref{sec:metrics}; this appendix adds the terms that appear only inside the axis identities: the recovery area $RA$, the graded-set areas $\mathrm{AUC}_{\mathcal G}$ and $PA_{\mathcal G}$, and the cost correction $\delta$.

\paragraph{Identities.} The chain axes decompose exactly (verified numerically to $10^{-15}$):
\begin{align}
  D_2 &= C(1)+\bigl(1-C(1)\bigr)\,\tfrac{1}{3}\bigl(R+\tfrac{16}{17}\,RA\bigr), \label{eq:app-d2}\\
  D_3 &= \mathrm{AUC}_{\mathcal G}+PA_{\mathcal G}, \label{eq:app-d3}
\end{align}
together with $D_4=NG(17)\times\Phi$ (\cref{eq:d4}) and $D_7=\mathrm{AUC}^{C}-\delta$ (\cref{eq:d7}). In~\cref{eq:app-d2}, $R$ is the recovery rate of~\cref{sec:metrics} and $RA$ the recovery area (how much and how early K1 failures are repaired), so the identity separates first-try success $C(1)$ from recovery after a K1 failure; the per-task ladder of~\cref{eq:d2} gives 1 at K1, 0.647 at K2, $-1/51$ per later round, 0.353 at K17 and 0 if unsolved, and the recovery term accounts for 48--74\% of D2 across systems. In~\cref{eq:app-d3}, $\mathrm{AUC}_{\mathcal G}$ is the binary coverage area on the twelve graded tasks and $PA_{\mathcal G}$ the partial-score area accrued before success or while unsolved. In~\cref{eq:d7}, $\delta\ge 0$ is the cost correction for the steps of successful episodes, recorded extra attempts (each charged one step limit) and truncation charge-back (unexecuted steps of failed episodes cut short by the reasoning budget, charged at the full limit). The ratios of $1-D_6$ reproduce the paired geometric-mean step ratios of~\cref{tab:app-cost}. \Cref{tab:app-decomp} gives the per-system components.

\begin{table}[t]
  \caption{\textbf{Per-system decomposition of the four chain axes.} Components of~\cref{eq:app-d2,eq:app-d3,eq:d4,eq:d7}; Sonnet values are observed snapshots (three unfinished chains). The K1-baseline variant of D4 (gain measured from $\bar q_1$ instead of $\bar q_0$) is 0.669 / 0.490 / 0.478 / 0.468; the difference is the K0$\to$K1 share quoted in~\cref{sec:exp-curves}.}
  \label{tab:app-decomp}
  \tablestyle{4pt}{1.08}
  \begin{tabular}{l z{34} z{34} z{34} z{34}}
    \toprule
    Quantity & Astra & Sol & Opus & Sonnet \\
    \midrule
    $C(1)$                 & 0.333 & 0.222 & 0.111 & 0.111 \\
    $C(17)$                & 0.833 & 0.667 & 0.722 & 0.611 \\
    $\mathrm{AUC}^{C}$     & 0.752 & 0.572 & 0.471 & 0.464 \\
    D2                     & 0.639 & 0.487 & 0.435 & 0.395 \\
    \midrule
    $\mathrm{AUC}_{\mathcal G}$ & 0.745 & 0.559 & 0.461 & 0.387 \\
    $PA_{\mathcal G}$      & 0.050 & 0.098 & 0.115 & 0.140 \\
    D3                     & 0.795 & 0.657 & 0.576 & 0.527 \\
    \midrule
    $NG(17)$               & 0.791 & 0.577 & 0.720 & 0.663 \\
    $\Phi$                 & 0.895 & 0.841 & 0.683 & 0.718 \\
    D4                     & 0.709 & 0.486 & 0.492 & 0.476 \\
    \midrule
    $\delta$               & 0.049 & 0.033 & 0.052 & 0.037 \\
    D7                     & 0.703 & 0.539 & 0.419 & 0.427 \\
    \bottomrule
  \end{tabular}
\end{table}

\paragraph{Composite.} $\bar A$ is the permutation-averaged radar area of~\cref{eq:area}; the equal-weight values 0.3268 / 0.2124 / 0.1425 / 0.1276 correspond to an equivalent radius $\sqrt{\bar A}$ of 0.572 / 0.461 / 0.378 / 0.357. The cluster-downweighted variant gives D2, D3, D4 and D7 weight $1/4$ each (the four together weigh as one axis) and D1, D6 weight 1: $\bar A$ = 0.2154 / 0.1594 / 0.0876 / 0.0787 with 95\% intervals [0.126, 0.321] / [0.083, 0.254] / [0.044, 0.152] / [0.037, 0.139], under which $P(\text{Sol}>\text{Opus})=0.994$ and $P(\text{Opus}>\text{Sonnet})=0.690$ (\cref{tab:area}).

\begin{table}[t]
  \caption{\textbf{Bootstrap covariation of the six axes.} Within-system Spearman correlation of axis scores across bootstrap resamples, averaged over the four systems. D2, D3, D4 and D7 move together with the first-success round; D1 and D6 are the two separate axes.}
  \label{tab:app-cov}
  \tablestyle{3.5pt}{1.08}
  \begin{tabular}{l z{26} z{26} z{26} z{26} z{26} z{26}}
    \toprule
         & D1 & D2 & D3 & D4 & D6 & D7 \\
    \midrule
    D1   & 1 & 0.38 & 0.26 & $-$0.03 & 0.35 & 0.31 \\
    D2   &   & 1    & 0.69 & 0.81    & 0.12 & 0.93 \\
    D3   &   &      & 1    & 0.70    & $-$0.03 & 0.74 \\
    D4   &   &      &      & 1       & $-$0.06 & 0.87 \\
    D6   &   &      &      &         & 1    & 0.09 \\
    D7   &   &      &      &         &      & 1 \\
    \bottomrule
  \end{tabular}
\end{table}

\paragraph{Shared first-success-round signal.} \Cref{tab:app-cov} gives the bootstrap covariation; task-level within-system correlations are higher still (D2--D3 0.96, D2--D4 0.96, D2--D7 0.99, D3--D4 0.95, D3--D7 0.94, D4--D7 0.95; D1 with the cluster 0.11--0.45; D6 with the cluster 0.26--0.56). What is genuinely extra in each axis ($PA_{\mathcal G}$ in D3, the K0 headroom normalization in D4, $\delta$ in D7) is real but not separated between systems (every interval includes zero) and never changes the order. Equal weighting therefore inflates differences when the four axes agree (98\% of the Astra--Sol area gap comes from the cluster) and inflates noise when they disagree (Sol versus Opus: D2, D3 and D7 favor Sol, D4 favors Opus).

\begin{table*}[t]
  \caption{\textbf{Ring order and leave-one-axis-out.} Top: drawn polygon area over all 60 ring orders (first axis fixed, mirrors removed); the system order is identical in all 60. Bottom: permutation-averaged area with one axis removed (equal weight, five axes); the point-estimate order never changes.}
  \label{tab:app-robust}
  \tablestyle{5pt}{1.08}
  \begin{tabular}{l z{40} z{40} z{40} z{40} z{64} z{70}}
    \toprule
    & Astra & Sol & Opus & Sonnet & $P(\text{Sol}{>}\text{Opus})$ & $P(\text{Opus}{>}\text{Sonnet})$ \\
    \midrule
    Ring-order range (min) & 0.307 & 0.203 & 0.130 & 0.116 & & \\
    Ring-order range (max) & 0.349 & 0.222 & 0.155 & 0.140 & & \\
    Recommended order\textsuperscript{b} & 0.321 & 0.215 & 0.141 & 0.124 & & \\
    \midrule
    Drop D1 & 0.412 & 0.252 & 0.195 & 0.168 & 0.875 & 0.824 \\
    Drop D2 & 0.309 & 0.207 & 0.133 & 0.121 & 0.981 & 0.719 \\
    Drop D3 & 0.277 & 0.179 & 0.114 & 0.104 & 0.963 & 0.715 \\
    Drop D4 & 0.295 & 0.207 & 0.125 & 0.110 & 0.988 & 0.751 \\
    Drop D6 & 0.372 & 0.232 & 0.154 & 0.145 & 0.953 & 0.666 \\
    Drop D7 & 0.296 & 0.198 & 0.135 & 0.117 & 0.960 & 0.820 \\
    \bottomrule
  \end{tabular}
  \par\smallskip\footnotesize \textsuperscript{b}D1 $\to$ D4 $\to$ D6 $\to$ D2 $\to$ D3 $\to$ D7, the order with the smallest sum of adjacent bootstrap covariances (1.78); its drawn area is within 3\% of $\bar A$.
\end{table*}

\paragraph{Robustness.} \Cref{tab:app-robust} reports the ring-order sweep (drawn-area range over all 60 ring orders) and the leave-one-axis-out areas with their pairwise probabilities, summarized in~\cref{sec:exp-axes}. On the tasks whose K0 (or K0 and K1) episodes were untruncated for all four systems ($n{=}7$ and $5$), the equal-weight areas are 0.318 / 0.149 / 0.145 / 0.120 and 0.323 / 0.169 / 0.172 / 0.150, \ie Sol and Opus tie; .

\paragraph{Axis numbering.} The labels keep the numbering of the eight-axis design we started from, which is why they skip D5; the numbering gap is explained here. D5 (iteration stability) was dropped because it took nearly identical values for every evaluated system (0.929--0.944) and was the only axis that violated the monotonicity requirement that improving a single task result must never lower an axis; D8 (process diagnostics such as tool calls and tokens) was dropped because the clients log them in non-comparable units. Both were dropped before any cross-system comparison.

\section{Additional Results}
\label{app:additional}

\Cref{tab:app-pertask} lists, for every task and system, the zero-shot score, the first-success round and the best observed score behind the aggregate axes of~\cref{sec:exp-axes}.

% Generated from analysis/four_model_metrics/tasks.csv on 2026-10-13 (handoff_pertask_table.tex, pasted as is).
\begin{table*}[t]
  \caption{\textbf{Per-task results.} For each system and task: zero-shot score $q_{t,0}$ (K0), first-success round $T_t$ within the 17-round budget (-- if unsolved by K17) and best observed score $\max_k q_{t,k}$. $^{\dagger}$: chain unfinished at snapshot time (Sonnet; last observed rounds K15, K15, K11). Source: \texttt{analysis/four\_model\_metrics/tasks.csv}.}
  \label{tab:app-pertask}
  \centering
  \tablestyle{3pt}{1.05}\scriptsize
  \begin{tabular}{l rrr rrr rrr rrr}
    \toprule
    & \multicolumn{3}{c}{Astra} & \multicolumn{3}{c}{Sol} & \multicolumn{3}{c}{Opus} & \multicolumn{3}{c}{Sonnet} \\
    \cmidrule(lr){2-4} \cmidrule(lr){5-7} \cmidrule(lr){8-10} \cmidrule(lr){11-13}
    Task & $q_{t,0}$ & $T_t$ & best & $q_{t,0}$ & $T_t$ & best & $q_{t,0}$ & $T_t$ & best & $q_{t,0}$ & $T_t$ & best \\
    \midrule
    \texttt{arrange\_largest\_number} & 0.15 & K1 & 1 & 0.3 & K2 & 1 & 0 & K3 & 1 & 0.05 & K2 & 1 \\
    \texttt{classify\_objects\_by\_language} & 1 & K1 & 1 & 1 & K1 & 1 & 0 & K4 & 1 & 0.1 & K2 & 1 \\
    \texttt{cover\_blocks} & 0.15 & K1 & 1 & 1 & K3 & 1 & 0.3 & K10 & 1 & 0 & K9 & 1 \\
    \texttt{deposit\_coin} & 0 & K4 & 1 & 0 & -- & 0.2 & 0 & K15 & 1 & 0.2 & -- & 0.2 \\
    \texttt{fill\_pen\_holder} & 0 & K3 & 1 & 0 & K8 & 1 & 0 & -- & 0.4 & 0 & --$^{\dagger}$ & 0.4 \\
    \texttt{insert\_key} & 0.15 & -- & 0.15 & 0.15 & -- & 0.15 & 0 & -- & 0.15 & 0.15 & -- & 0.15 \\
    \texttt{match\_and\_pick\_from\_conveyor} & 1 & K1 & 1 & 1 & K1 & 1 & 1 & K1 & 1 & 0 & K1 & 1 \\
    \texttt{organize\_table} & 0 & K2 & 1 & 0.5 & -- & 0.5 & 0 & K14 & 1 & 0.25 & -- & 0.75 \\
    \texttt{pack\_objects\_into\_box} & 0.5 & K9 & 1 & 0.5 & K6 & 1 & 0 & K15 & 1 & 0 & --$^{\dagger}$ & 0.25 \\
    \texttt{play\_Xylophone} & 0 & K4 & 1 & 0 & K4 & 1 & 0 & -- & 0 & 0 & K7 & 1 \\
    \texttt{plug\_in\_charger} & 0 & K2 & 1 & 0 & -- & 0 & 0 & K10 & 1 & 0 & K7 & 1 \\
    \texttt{pour\_by\_language} & 0 & K5 & 1 & 0 & K7 & 1 & 0 & K4 & 1 & 0 & K13 & 1 \\
    \texttt{pour\_liquid\_into\_cup} & 0 & K2 & 1 & 0 & K5 & 1 & 0 & K3 & 1 & 0 & K4 & 1 \\
    \texttt{push\_T} & 0 & K3 & 1 & 0 & K1 & 1 & 0 & K8 & 1 & 0 & K8 & 1 \\
    \texttt{put\_bottles\_into\_dustbin} & 0.4 & K1 & 1 & 0.1 & K2 & 1 & 0.25 & K1 & 1 & 0.25 & K1 & 1 \\
    \texttt{stack\_blocks\_by\_language} & 1 & K1 & 1 & 0.2 & K1 & 1 & 0 & K2 & 1 & 1 & K2 & 1 \\
    \texttt{store\_tools\_in\_toolbox} & 0 & -- & 0.5 & 0 & -- & 0.25 & 0 & -- & 0 & 0 & --$^{\dagger}$ & 0 \\
    \texttt{swap\_blocks} & 0 & -- & 0 & 0 & -- & 0 & 0 & -- & 0 & 0 & -- & 0 \\
    \bottomrule
  \end{tabular}
\end{table*}

\begin{table}[t]
  \caption{\textbf{Task coverage $C(K)$ per round, 18 tasks.} Number of tasks whose first native success occurred at or before round $K$. Sonnet values from K12 onward are lower bounds (three unfinished chains; upper bound 14/18 at K17).}
  \label{tab:app-coverage}
  \tablestyle{5pt}{1.0}
  \begin{tabular}{z{14} z{30} z{30} z{30} z{30}}
    \toprule
    $K$ & Astra & Sol & Opus & Sonnet \\
    \midrule
    1  & 6  & 4  & 2  & 2 \\
    2  & 9  & 6  & 3  & 5 \\
    3  & 11 & 7  & 5  & 5 \\
    4  & 13 & 8  & 7  & 6 \\
    5  & 14 & 9  & 7  & 6 \\
    6  & 14 & 10 & 7  & 6 \\
    7  & 14 & 11 & 7  & 8 \\
    8  & 14 & 12 & 8  & 9 \\
    9  & 15 & 12 & 8  & 10 \\
    10 & 15 & 12 & 10 & 10 \\
    11 & 15 & 12 & 10 & 10 \\
    12 & 15 & 12 & 10 & $\ge$10 \\
    13 & 15 & 12 & 10 & $\ge$11 \\
    14 & 15 & 12 & 11 & $\ge$11 \\
    15 & 15 & 12 & 13 & $\ge$11 \\
    16 & 15 & 12 & 13 & $\ge$11 \\
    17 & 15 & 12 & 13 & $\ge$11 \\
    \bottomrule
  \end{tabular}
\end{table}

\paragraph{Coverage and growth-shape details.} \Cref{tab:app-coverage} tabulates $C(K)$: tasks solved by K3 / K6 / K17 number 11 / 14 / 15 (Astra), 7 / 10 / 12 (Sol), 5 / 7 / 13 (Opus) and 5 / 6 / 11 (Sonnet). Opus's six tasks solved after K6 are \texttt{push\_T} (K8), \texttt{cover\_blocks} and \texttt{plug\_in\_charger} (K10), \texttt{organize\_table} (K14), and \texttt{pack\_objects\_into\_box} and \texttt{deposit\_coin} (K15). Quantities not reported in the body: K1 mean score $\bar q_1$ = 0.403 / 0.297 / 0.156 / 0.167, best-so-far mean score at K17 0.869 / 0.728 / 0.753 / 0.708, mean first-success round over solved tasks 2.67 / 3.42 / 6.92 / 5.09, and tasks improved / tied / worsened from K0 to the last observation 12 / 6 / 0, 9 / 8 / 1, 14 / 4 / 0 and 13 / 5 / 0. The increment uniformity of~\cref{sec:exp-growth} is read up to the 90\% crossing; at the 95\% and 100\% thresholds it is 0.593 / 0.836 / 0.555 / 0.448 and 0.389 / 0.706 / 0.555 / 0.448, so Astra's late plateau and wobble lower its uniformity and ``uniform growth'' holds for it only up to the 90\% crossing.

\begin{table}[t]
  \caption{\textbf{Resource and cost readings.} Steps are native control steps of K1--K17 episodes; only Astra's extra attempts have recorded step counts (0 means not recorded, not no extra attempts). Wall-clock is per-episode native time summed over parallel episodes. Token readings use different meters per vendor and are not comparable.}
  \label{tab:app-cost}
  \tablestyle{2.5pt}{1.08}
  \begin{tabular}{y{88} z{28} z{28} z{28} z{28}}
    \toprule
    Quantity & Astra & Sol & Opus & Sonnet \\
    \midrule
    Canonical episodes (K0--K17) & 109 & 161 & 193 & 183 \\
    Recorded K1--K17 steps & 63\,840 & 92\,442 & 121\,319 & 118\,019 \\
    \quad of which extra-attempt steps & 9\,555 & 0 & 0 & 0 \\
    Recorded wall-clock (min) & 10\,509 & 6\,806 & 13\,486 & 14\,005 \\
    Tasks solved within 5000 steps & 14/18 & 10/18 & 10/18 & 9/18 \\
    Tasks solved within 5\,h / 10\,h & 10 / 12 & 9 / 10 & 7 / 8 & 6 / 9 \\
    Median first-success steps, 9 common tasks & 407 & 491 & 601 & 653 \\
    Paired step ratio vs.\ Astra & 1.000 & 1.048 & 1.140 & 1.231 \\
    Known extra attempts & 13 & 9 & 21 & 37 \\
    Episode duration P50 / P90 (min) & 91 / 197 & 47 / 89 & 72 / 130 & 79 / 144 \\
    Output tokens (M) & 1.83\textsuperscript{c} & 5.59 & 12.7\textsuperscript{d} & 35.4\textsuperscript{d} \\
    \bottomrule
  \end{tabular}
  \par\smallskip\footnotesize \textsuperscript{c}Measured on 71 of 91 episodes plus 0.60\,M estimated. \textsuperscript{d}Terminal estimates, no input tokens. Dollar cost is not available for any system.
\end{table}

\paragraph{Cost.} \Cref{tab:app-cost} collects the resource readings behind D6 and D7. Astra's step total includes 9\,555 steps from its 13 recorded extra attempts; the 9 / 21 / 37 extra attempts known for Sol, Opus and Sonnet from the session audit have no recorded step counts, so their totals are lower bounds. The wall-clock totals are per-episode native time summed over parallel runs, include waiting and use vendor-specific timing boundaries, so they are neither calendar time nor a speed ranking; token and dollar costs are likewise not four-way comparable (\cref{sec:exp-axes}). Under the plain convention (measured canonical-chain steps only, no imputed extra attempts) D7 would be 0.731 / 0.549 / 0.451 / 0.445 and the Opus/Sonnet order flips, which is one of the reasons the pair is reported as undecidable.

\paragraph{Ablation layout schedule.} The six ablation tasks are \texttt{push\_T}, \texttt{plug\_in\_charger}, \texttt{deposit\_coin}, \texttt{play\_Xylophone}, \texttt{pour\_by\_language} and \texttt{pour\_liquid\_into\_cup}, each with two replicate chains per group. The scene layout changes every round with the same sequence in every group: replicate 1 cycles layouts 1--6 over K1--K6 and replicate 2 layouts 7--12; A0F keeps its first layout throughout (layout 1 for replicate 1, layout 7 for replicate 2). Held-out layouts 13--17 are used only by the frozen tests (\cref{tab:app-frozen}).

\begin{table}[t]
  \caption{\textbf{Per-round online success in the Astra ablation.} Successes out of 12 chains per group and round (K1--K6 run in full, no first-success stop); A4R has 11 chains at K6. A0F trains on a fixed, already-seen layout and is descriptive only.}
  \label{tab:app-ablation-rounds}
  \tablestyle{3pt}{1.0}
  \begin{tabular}{z{14} z{26} z{26} z{26} z{26} z{26} z{26}}
    \toprule
    $K$ & A0 & A0F & A1 & A2 & A4R & A5 \\
    \midrule
    1 & 1 & 1 & 1 & 0 & 0 & 1 \\
    2 & 2 & 3 & 1 & 2 & 1 & 2 \\
    3 & 6 & 6 & 3 & 2 & 2 & 1 \\
    4 & 6 & 8 & 4 & 2 & 7 & 0 \\
    5 & 5 & 7 & 3 & 2 & 3 & 0 \\
    6 & 4 & 7 & 5 & 1 & 6/11 & 3 \\
    \midrule
    K4--K6 & 15/36 & 22/36 & 12/36 & 5/36 & 16/35 & 3/36 \\
    \bottomrule
  \end{tabular}
\end{table}

\paragraph{Ablation per round.} \Cref{tab:app-ablation-rounds} gives the per-round success counts behind the late-round rates of~\cref{tab:ablation} and the paired contrasts of~\cref{fig:ablation}.

\begin{table}[t]
  \caption{\textbf{Frozen held-out test of Astra K6 workspaces.} Each source chain's K6-revised workspace is frozen and run once on each of five held-out layouts (13--17) with no revision and no outcome feedback; 12 sources $\times$ 5 layouts for the complete groups. HO-A1 and HO-A2 are incomplete and not comparable with the core groups.}
  \label{tab:app-frozen}
  \tablestyle{2.5pt}{1.08}
  \begin{tabular}{y{38} y{78} z{30} z{28} z{26}}
    \toprule
    Condition & Semantics & Sources & Succ./$n$ & Rate \\
    \midrule
    E3-full  & A0 workspaces; test agent may read prior-round raw records & 12 & 23/60 & 38.3\% \\
    E3-notes & A0 workspaces; workspace files only & 12 & 25/60 & 41.7\% \\
    HO-A0F   & fixed-layout (A0F) workspaces on new layouts & 12 & 27/60 & 45.0\% \\
    HO-A1    & A1 (no images) workspaces; incomplete & 9 (6) & 13/35 & 37.1\% \\
    HO-A2    & A2 (no outcome detail) workspaces; incomplete & 6 (1) & 5/21 & 23.8\% \\
    \bottomrule
  \end{tabular}
\end{table}

\paragraph{Fixed and held-out layouts.} \Cref{tab:app-frozen} gives the frozen held-out test (Astra only, six ablation tasks): 60 episodes per complete condition, no revision, no feedback. A0F has the highest online late-round rate (22/36, 61\%) but is scored on a layout it has already seen: on its seen layouts it succeeds in 14/16 rounds (88\%) against 5/16 (31\%) for A0, whereas its frozen K6 workspaces succeed in 27/60 (45\%) on the five held-out layouts. The layout double difference (A0F seen $-$ A0F new) $-$ (A0 seen $-$ A0 new) is $+43.75$\,pp, 95\% CI [$+22.5$, $+73.75$] on four tasks (task-cluster bootstrap, $B{=}20\,000$, exploratory), with a test-channel confound that prevents attributing all of it to memorization; fixed-layout training scores are therefore consistent with scene memorization and are not used to select a configuration. The same test shows no detectable harm from full history at test time: the A0 K6 workspaces reach 25/60 (41.7\%) when the test agent reads workspace files only (E3-notes) and 23/60 (38.3\%) when it can also read the raw prior-round records (E3-full), a difference of $-3.3$\,pp [$-25$, $+15$], an interval containing zero that is not evidence of equivalence. Cross-layout robustness of the frozen sources (number of sources succeeding on 0 / 1 / 2 / 3 / 4 / 5 of the five layouts): E3-full 4 / 2 / 1 / 3 / 0 / 2, E3-notes 4 / 1 / 1 / 4 / 0 / 2, HO-A0F 2 / 1 / 5 / 2 / 0 / 2. A0's online K4--K6 rate (41.7\%) and its frozen held-out rates (38--42\%) are close, which is why the body reads changing-layout online rates as a proxy for new-layout performance.
% The master doc gives the frozen contrast as "-3 pp, CI about [-17, +11]"; the repo JSON (M34) gives -3.33 [-25, +15]. Repo value used.

\section{Capability-Source Analysis Details}
\label{app:pca}

This appendix documents the framework for relating the composite $\bar A$ to public-benchmark abilities. It follows the observational approach of~\citet{ruan2024observational}, with the \methodname composite in place of a downstream benchmark score. The analysis is exploratory and incomplete: nothing in it is a result, and no loading is interpreted until the benchmark set, the system set and the component count are frozen.

\begin{figure*}[tb]
  \centering
  \IfFileExists{assets/fig_pca_heatmap_provisional.png}{\includegraphics[width=\textwidth]{assets/fig_pca_heatmap_provisional.png}}{}
  \caption{\textbf{Provisional: PCA loadings of eight public benchmark families on five components (six-system PCA).} Each cell is the eigenvector coefficient of a benchmark family (or named sub-task) on a component, not an RSI effect size; the row percentage is the share of benchmark-score variance explained (PC1 44.0\%, PC2 31.4\%, PC3 15.6\%, PC4 7.0\%, PC5 2.0\%). Columns were selected with the four RSI-labeled systems in mind; all six systems are scored at their maximum public setting. Whether any component predicts $\bar A$ is not yet tested; no loading is interpreted until the column and model sets are frozen. Descriptive and exploratory; leaderboard snapshot 2026-10-13.}
  \label{fig:pca}
\end{figure*}

\paragraph{Three objects.} Treating public evaluations as observable capability indicators~\cite{ruan2024observational}, we collect public benchmark scores for the same systems and factor them, keeping three objects separate: (i)~\emph{loadings}, from a PCA over benchmark families, which say which benchmarks move together across systems; (ii)~\emph{per-system component scores}, the position of each system on each component; and (iii)~a \emph{fit} of the composite $\bar A$ (\cref{tab:area}) on the component scores, validated leave-one-out, which says whether any component predicts the embodied improvement. Only (iii) speaks to the source of RSI capability: any statement of the form ``the composite tracks ability X'' requires a held-out system or a replicated chain on which the prediction is checked, and until then the decomposition remains a description of the leaderboard geometry of four to six systems.

\paragraph{Benchmark set.} Candidate benchmark families named in planning for the PCA column set were Terminal-Bench~\cite{merrill2026terminalbench}, Humanity's Last Exam~\cite{phan2025hle}, LiveBench~\cite{white2024livebench} and GDPval~\cite{patwardhan2025gdpval}; OSWorld~\cite{xie2024osworld} and SciCode~\cite{tian2024scicode} were considered but have not been used, nor have CritPt, AA-Briefcase and AA-Omniscience. Two exploratory column sets have been tried: (i)~six columns combining four LiveBench sub-scores (reasoning: logic with navigation; language: plot unscrambling; instruction following: paraphrase; coding: code generation) with FrontierCode 1.1 and Terminal-Bench 4.0; (ii)~eight benchmark families, AutomationBench-AA, GDPval-AA v2.1, Humanity's Last Exam without tools, AA-LCR v1.1, FrontierCode 1.1 Extended, LiveBench instruction following, Terminal-Bench Science 0.1 and Terminal-Bench 4.0 Software, the set drawn in~\cref{fig:pca}. The final column set is fixed here, not in the body. 

\paragraph{Model set.} Set (i) has three components and therefore four systems; set (ii) is a six-system PCA of which only the four \methodname systems carry a composite label, so step (iii) has not been run and any fit on four points will be descriptive at best. Leaderboard scores were taken at each vendor's maximum public reasoning setting, whereas the benchmark runs used xhigh / xhigh / high / xhigh; the mapping must be disclosed once the analysis is frozen. 

\paragraph{PCA settings and provisional state.}  Exploratory values: set (i) gives PC1 / PC2 / PC3 = 90.2 / 7.6 / 2.2\% of variance and a leave-one-out MAE of 0.059 for a PC1 regression against an unspecified target; with four labeled systems a first component explaining 90\% of variance is close to degenerate. Set (ii), drawn in~\cref{fig:pca}, is reduced to five components over six systems (provisionally, PC1 explains 44.0\% of the benchmark variance; ). In both sets the loadings are descriptive coefficients, not effects on the composite, and the sign convention has not been fixed.

\paragraph{Hypotheses.} Four abilities are candidate explanations, stated as hypotheses only: coding (writing, modifying and debugging the policy), spatial reasoning (locating objects and their relations from images), logical and causal reasoning (turning failure feedback into a revised strategy) and long-context handling (exploiting the accumulated multi-round history). Which of them, if any, the fitted model favors is left to the final analysis.

\paragraph{What remains to be run.} Freeze the column set and the system set; recompute the PCA with a stated standardization and component count; compute the per-system component scores; fit $\bar A$ on them leave-one-out; and report the three objects apart, with the configuration mapping between leaderboard settings and benchmark runs.
